# Supplementary material for: BreachRadar: Automatic Detection of Points-of-Compromise
Source: arXiv:2009.11751 source file (2020-09-24)
Supplement: Supplementary file 1 [file appendixA.tex]

\appendix[Fraud Label Delays] \label{appendix:labeldelays}% This is Appendix A
The availability of fraud labels is an obvious requirement of the procedure described in this work. Without fraud labels, or with a significant delay between the transaction date and the date in which the fraud label was added, our ability to minimize eventual losses is severely restricted. Therefore, we present a preliminary analysis on whether these labels are available in a reasonable time frame. 

Figure \ref{fig:labeldelay} shows the distribution that relates the number of fraudulent transactions and the number of days the respective label was assigned. We can see that the number of days that a typical label is delayed is very small; while it might be initially surprising, the reality is that several systems try to detect whether a transaction is fraudulent in real-time. Financial institutions then either abort the transaction or call the card owner in order to validate the purchase.

Furthermore, note that once a card has been cloned and is successfully used in a fraudulent transaction, fraudsters will typically use that opportunity to spend all the available funds as fast as possible, before the rightful owners are able to communicate the unauthorized transactions to their bank. As a consequence, with a nearly empty or even over-drafted account, customers are quick to report these transactions to their banking institution.

\begin{figure}[ht] 
  \centering 
  \includegraphics[width=0.40\textwidth,trim=0mm 2mm 0mm 3mm, clip]{FIG/fraudDelay.eps} 
  \caption{\textbf{Most labels are available shortly after the transaction.} (actual counts removed for privacy)}
  \label{fig:labeldelay}
\end{figure}
